# Supplementary material for: DOGE: Differentiable Bezier Graph Optimization for Road Network Extraction
Source: arXiv:2511.19850 source file (2025-11-25)
Supplement: Supplementary file 1 [file X_suppl.tex]

\appendix

\setcounter{figure}{0}
\setcounter{table}{0}
\setcounter{equation}{0}

\section{DOGE Global Optimization Framework}

\subsection{Full Algorithm of DOGE}
% \subsubsection*{Notes}
% \begin{itemize}
%     \item Presents the complete pseudocode for DOGE, which is an extended version of Algorithm 1 in the main paper.
%     \item Includes details on initialization, DiffAlign iterations, the invocation frequency of TopoAdapt, curve update procedures, the sequence of loss calculations, and the sampling/rendering pipeline.
% \end{itemize}

\begin{algorithm}
	\caption{Detailed Algorithm of DOGE}
	\label{alg:full_doge_algorithm}
	\KwIn{$I_{target}$: Target satellite image; $N_{epochs}$: Number of training epochs}
	\KwOut{$\mathcal{G}^*$: The optimized road graph}

	$\mathcal{S} \leftarrow \text{SAM2}(I_{target})$;
	$\mathcal{G}_0=\{V_0, E_0, \theta_0\} \leftarrow \text{InitializeGraph}(\mathcal{S})$;

	\For{$t = 0$ \KwTo $N_{epochs}-1$}
	{
		% TopoAdapt: Connectivity Enhancement
		\If{$t > T_{warmup}$}
		{
			% Merge nearby nodes
			\While{exists pair $(u, v) \in V_t \times V_t$ s.t. $u \neq v$ and $||u.p - v.p|| < \epsilon_{merge}$}
			{
				$V_t, E_t \leftarrow \text{MergeNodes}(V_t, E_t, u, v)$;
			}
			
			% Create T-junctions
			\While{exists $(v, e) \in V_t \times E_t$ s.t. $v \notin \{e.start, e.end\}$ and $\text{dist}(v, e) < \epsilon_{merge}$}
			{
				$V_t, E_t \leftarrow \text{CreateTJunction}(V_t, E_t, v, e)$;
			}
		}
		
		% TopoAdapt: Graph Simplification
		\For{$v \in V_t$ where $v.degree = 2$ and $v.age > T_{collinear\_age}$}{
			$\{e_i, e_j\} \leftarrow \text{GetIncidentEdges}(v)$;
			\If{$\text{angle}(e_i, e_j) > \theta_{collinear}$}
			{
				$V_t, E_t \leftarrow \text{MergeCollinearEdges}(V_t, E_t, v, e_i, e_j)$;
			}
		}
		
		% TopoAdapt: Pruning
		$E_t \leftarrow \text{PruneInvalidEdges}(E_t)$;
		$V_t \leftarrow \text{RemoveDanglingNodes}(V_t)$;

		% TopoAdapt: Road Addition
		\If{$t \pmod{T_{add\_road}} = 0$}
		{
			$V_t, E_t \leftarrow \text{AddRoadsAtUnfit}(V_t, E_t, \mathcal{S}, \mathcal{R}(\mathcal{G}_t))$;
		}

		% DiffAlign Step
		$\mathcal{L} \leftarrow \text{ComputeLoss}(\mathcal{R}(\mathcal{G}_t), \mathcal{S}, \mathcal{G}_t)$;
		$\theta_{t+1} \leftarrow \text{Adam}(\theta_t, \nabla_{\theta_t} \mathcal{L})$;
		$\mathcal{G}_{t+1} \leftarrow (V_t, E_t, \theta_{t+1})$;
	}

	\Return{$\mathcal{G}_{N_{epochs}}$};
\end{algorithm}

\paragraph{Graph Initialization.}
The optimization process begins with a sparse initialization of the B\'{e}zier graph $\mathcal{G}_0$. This procedure first identifies all non-background pixels in the target segmentation $\mathcal{S}$. From this set of candidate pixels, a predetermined number of locations are randomly sampled to serve as centers for new road segments. For each sampled point, a straight B\'{e}zier edge is created with a predefined initial length and width, and assigned a random orientation. This results in a disconnected set of edges that provides a coarse, distributed coverage of the road regions in $\mathcal{S}$, serving as the starting point for the iterative refinement process.

\paragraph{TopoAdapt Operations.}
Instead of being a monolithic step invoked at a fixed interval, \textit{TopoAdapt} is a collection of discrete operators applied dynamically based on the state of the graph. The workflow is as follows:
\begin{itemize}
    \item \textbf{Road Addition:} New edges are periodically introduced in under-covered regions of the segmentation. For instance, this operation can be triggered every 20 global steps to ensure the graph grows to match the target.
    \item \textbf{Pruning:} In every iteration, edges that are geometrically implausible, such as being too short or too thin, are pruned. The pruning thresholds become stricter after an initial grace period, for example, after 20 iterations of an edge's existence, to allow new edges to stabilize.
    \item \textbf{Connectivity Enhancement:} After an initial warm-up period, a connectivity function is executed. It efficiently identifies and creates T-junctions and merges nearby nodes using a spatial grid for acceleration. These operations are only applied to nodes and edges that have existed for a minimum number of iterations, such as 15, ensuring that only mature parts of the graph are modified.
    \item \textbf{Collinear Merging:} Degree-2 nodes that form nearly straight lines are simplified. This operation is also conditional on the node's age; for example, a node must exist for more than 60 iterations, preventing the premature merging of newly formed, yet-to-be-optimized junctions.
\end{itemize}
This stateful, condition-driven approach allows the graph to evolve more organically, applying topological changes only when components are geometrically stable.

\paragraph{Accelerated Proximity Queries.}
To efficiently perform proximity-based topological operations such as node merging and T-junction creation, a naive all-pairs check would be computationally prohibitive, with a complexity of $O(N^2)$ or worse. We accelerate these queries by employing a spatial grid. Before executing connectivity enhancements, a grid is constructed where each cell stores the nodes and edges that fall within its boundaries. When searching for neighbors for a given node or edge, the search is restricted to its host cell and the immediately adjacent cells. This spatial partitioning drastically reduces the search space, making the process scalable for large and dense road networks. Furthermore, distance calculations for large batches of candidate pairs are vectorized to leverage GPU parallelism for maximum efficiency.

\subsection{Hyperparameters of DiffAlign and TopoAdapt}
Our framework is designed to be robust, utilizing a single, fixed set of hyperparameters across all datasets without the need for dataset-specific tuning. This demonstrates the generalization capability of our approach. The key parameters for both the differentiable optimization (\textit{DiffAlign}) and the discrete topological refinement (\textit{TopoAdapt}) are detailed in \cref{tab:hyperparameters}.

\begin{table}[h]
	   \centering
	   \small
	   \caption{Hyperparameters for the DOGE framework. All parameters are fixed across all experiments.}
	   \label{tab:hyperparameters}
	   \setlength{\tabcolsep}{4pt}
	   \begin{tabular}{@{}l l c@{}}
	   \toprule
	   \textbf{Module} & \textbf{Hyperparameter} & \textbf{Value} \\
	   \midrule
	   \textit{DiffAlign} & Learning Rate $\eta$ & $1 \times 10^{-3}$ \\
	   & $\lambda_{\text{cover}}$ (Coverage Loss) & 1.0 \\
	   & $\lambda_{\text{overlap}}$ (Overlap Loss) & 0.3 \\
	   & $\lambda_{G1}$ (G1 Continuity Loss) & 0.012 \\
	   & $\lambda_{\text{offset}}$ (Offset Loss) & $6\times 10^{-3}$ \\
	   & $\lambda_{\text{spacing}}$ (Spacing Loss) & $6\times 10^{-3}$ \\
	   & $T_{G1}$ (G1 Angle Threshold) & $90^{\circ}$ \\
	   & $\tau_d$ (Max Offset Ratio) & 0.75 \\
	   \midrule
	   \textit{TopoAdapt} & Road Addition Frequency & 20 iterations \\
	   & Connectivity/Merge Min. Age & 15 iterations \\
	   & Collinear Merge Min. Age & 60 iterations \\
	   & $\epsilon_{\text{merge}}$ (Node Merge/Snap Distance) & 4.0m \\
	   & $\epsilon_{\text{angle}}$ (Collinear Merge Angle) & $170^{\circ}$ \\
	   & Min Edge Length/Width (Pruning) & 0.6m / 0.3m \\
	   & Min Unfit Area (Road Addition) & 50 $m^2$ \\
	   \bottomrule
	   \end{tabular}
\end{table}

\subsection{B\'{e}zier Graph Serialization and Sampling}

\paragraph{Serialization to Polygons.}
To render the B\'{e}zier graph using a differentiable rasterizer like DiffVG, each curve must be converted into a closed polygon. For a given B\'{e}zier edge $e_k$ with width $w_k$, we first sample a sequence of points along its centerline $\boldsymbol{C}_k(t)$ for $t \in [0, 1]$. At each sampled point, we compute the curve's normal vector. By offsetting the centerline points by $\pm w_k/2$ along their respective normals, we generate two parallel boundary polylines. These two polylines are then connected at their ends to form a closed polygon that accurately approximates the road segment's shape, which can then be processed by the rasterizer.

\paragraph{Sampling B\'{e}zier Curves to Polylines.}
To evaluate the topological quality of the extracted graphs using standard metrics like APLS and TOPO, we must convert our continuous B\'{e}zier graph representation into discrete polylines. Since these metrics compare graph structures based on node positions and edge paths, we perform a high-resolution discretization of each cubic B\'{e}zier edge.
For every edge $e$ defined by control points $\mathbf{P}_0, \mathbf{P}_1, \mathbf{P}_2, \mathbf{P}_3$, we sample points along the curve at a fixed interval of 1 meter. The length of the curve is first estimated using a 100-point piecewise linear approximation. Based on this length, we calculate the number of segments required and uniformly sample the parameter $t \in [0, 1]$ to generate the corresponding sequence of GPS coordinates. This dense sampling ensures that the curvature and connectivity of the predicted road network are accurately preserved in the graph format required for metric calculation.

\paragraph{DiffVG Rendering Settings.}
Our framework uses DiffVG for differentiable rendering. The scene is rendered onto a canvas of a specified resolution. Each serialized road polygon is drawn with a solid color and full opacity. We use 4 samples per pixel (spp) for anti-aliasing to ensure smooth gradients during backpropagation. The rendering process is configured to be fully differentiable with respect to the control point positions and widths of the B\'{e}zier curves.

\subsection{Early-Stopping Strategy in DOGE}
We implement an early-stopping mechanism to prevent redundant computation. The optimization process is halted if the coverage loss plateaus and the topology remains unchanged for a predefined number of epochs, ensuring the B\'{e}zier graph has stably converged to the target road network.

\section{Modified SAM2 Architecture and Training Details}

\subsection{Network Architecture Overview}
To adapt the Segment Anything Model 2 (SAM2) for high-resolution road segmentation in satellite imagery, we design a dual-branch architecture that effectively integrates pre-trained semantic knowledge with fine-grained spatial details. The complete pipeline integrates three key stages:
\begin{enumerate}
    \item Modified SAM2 Backbone (Semantic Stream): We utilize the Hiera-L backbone from SAM2 to extract robust high-level semantic representations, adapted for satellite image patches via dynamic positional embedding adjustments.
    \item Lightweight Auxiliary Encoder (Spatial Stream): Running in parallel, a ResNet-18 encoder captures low-level texture and boundary information often lost in patch-based transformer processing.
    \item Multi-scale Fusion: The \texttt{Multiscale}\allowbreak\texttt{Fusion}\allowbreak\texttt{UNet}\allowbreak\texttt{Decoder} acts as the bridge, fusing features from both streams. It combines deep semantics from SAM2 with spatial hierarchies from the auxiliary encoder via skip connections at corresponding resolutions ($1/16, 1/8, 1/4$) to generate the final mask.
\end{enumerate}
This collaborative design ensures the model retains the generalization power of SAM2 while achieving the pixel-level precision required for road network extraction.

\subsection{Modified SAM2 Backbone}
We utilize the \texttt{sam2.1\_hiera\_l} (Large) configuration as our primary backbone. The Hiera architecture processes images through four hierarchical stages with embedding dimension of 144 and global attention blocks.
\paragraph{Resolution Adaptation.} Standard SAM2 models are optimized for $1024 \times 1024$ inputs. For efficient processing of satellite patches (typically $256 \times 256$ for SpaceNet or $512 \times 512$ for CityScale), we implement a dynamic configuration adapter. This module recalculates the \textit{Rotary Position Embedding} (RoPE) parameters to match the scaled-down feature map dimensions, enabling the heavy backbone to process smaller patches without interpolation artifacts.

\subsection{Lightweight Auxiliary Encoder}
To supplement the semantic features from SAM2, we employ a ResNet-18 based auxiliary encoder. This lightweight branch specifically targets spatial hierarchy recovery. It extracts features from the early stages of a pre-trained ResNet-18 to capture texture and boundary information. The structure of this auxiliary branch is detailed in Table~\ref{tab:aux_encoder}.

\begin{table}[h]
    \centering
    \small
    \caption{Structure of the Lightweight Auxiliary Encoder (ResNet-18 based) for $256 \times 256$ input. Output sizes are denoted as $C \times H \times W$.}
    \label{tab:aux_encoder}
    \setlength{\tabcolsep}{4pt}
    \begin{tabular}{@{}l|l|c@{}}
    \toprule
    \textbf{Layer Name} & \textbf{Structure / Operations} & \textbf{Output Tensor} \\
    \midrule
    Input & - & $3 \times 256 \times 256$ \\
    Initial & Conv$7{\times}7$, BN, ReLU, MaxPool & $64 \times 64 \times 64$ \\
    Layer 1 & BasicBlock $\times 2$ & $64 \times 64 \times 64$ \\
    Layer 2 & BasicBlock $\times 2$, Stride 2 & $128 \times 32 \times 32$ \\
    \bottomrule
    \end{tabular}
\end{table}

\subsection{Multi-scale Fusion and Skip Connections}
A key innovation in our design is the \texttt{Multiscale}\allowbreak\texttt{Fusion}\allowbreak\texttt{UNet}\allowbreak\texttt{Decoder}, which integrates information from three distinct sources via skip connections. The data flow is explicitly designed to merge semantic context with spatial precision:

\begin{enumerate}
    \item \textbf{Deep Semantics (SAM2 Backbone):} The final output of the SAM2 Hiera backbone at $1/16$ scale ($16 \times 16$). The original 1152 channels are reduced to 256 via a $1 \times 1$ convolution before entering the decoder.
    \item \textbf{SAM2 FPN Features:} Intermediate feature maps from the SAM2 Feature Pyramid Network at $1/8$ scale ($32 \times 32$, 256 ch) and $1/4$ scale ($64 \times 64$, 256 ch).
    \item \textbf{Auxiliary Spatial Features:} Features from the Lightweight Auxiliary Encoder at corresponding resolutions: Layer 2 ($32 \times 32$, 128 ch) and Layer 1 ($64 \times 64$, 64 ch).
\end{enumerate}

\paragraph{Detailed Fusion Data Flow.}
We detail the network architecture and tensor transformations for the standard $256 \times 256$ input in \Cref{tab:decoder_arch}. The decoding process utilizes a multi-stage fusion strategy:
at the 32$\times$32 and 64$\times$64 resolutions, the decoder fuses features from three distinct sources: the upsampled features from the previous decoder stage, the corresponding skip connection from the SAM2 Feature Pyramid Network (FPN), and the hierarchical feature map from the Lightweight Auxiliary Encoder. These features are concatenated channel-wise and then processed by a DoubleConv block (Conv$3{\times}3$-LN-GELU $\times 2$) to effectively integrate context and reduce channel dimensionality. For the subsequent stages (128$\times$128 and 256$\times$256), the network follows a standard U-Net upsampling path to recover the full spatial resolution.

\begin{table}[h]
    \centering
    \footnotesize
    \caption{Architecture details of the Fusion U-Net Decoder with a $256 \times 256$ input. The ``Fusion'' operation integrates features from the SAM2 FPN and the Lightweight Auxiliary Encoder (Aux.), as detailed in the text.}
    \label{tab:decoder_arch}
    \setlength{\tabcolsep}{2pt}
    \begin{tabular}{@{}l l c@{}}
    \toprule
    \textbf{Layer Name} & \textbf{Structure / Operations} & \textbf{Output Tensor} \\
    \midrule
    Input & SAM2 Backbone Output & $256 \times 16 \times 16$ \\
    \midrule
    Decoder 1 & Upsample, Fusion (w/ Aux.), DoubleConv & $128 \times 32 \times 32$ \\
    Decoder 2 & Upsample, Fusion (w/ Aux.), DoubleConv & $64 \times 64 \times 64$ \\
    Decoder 3 & Upsample, DoubleConv & $32 \times 128 \times 128$ \\
    Decoder 4 & Upsample, DoubleConv & $16 \times 256 \times 256$ \\
    \midrule
    Output & Final Conv$1{\times}1$ & $1 \times 256 \times 256$ \\
    \bottomrule
    \end{tabular}
\end{table}

\subsection{Training Strategy and Optimization}
We implement the proposed framework using PyTorch Lightning and conduct training on NVIDIA GeForce RTX 4090 GPU. The training process is optimized as follows:

\paragraph{Optimizer and Scheduling.} We use the \textbf{AdamW} optimizer with a base learning rate of $4.45 \times 10^{-4}$. To effectively adapt the pre-trained SAM2 backbone while learning new spatial features, we employ a \textbf{layer-wise learning rate strategy}:
\begin{itemize}
    \item \textbf{SAM2 Backbone:} Learning rate scaled by $0.045\times$ to preserve pre-trained semantic knowledge.
    \item \textbf{Lightweight Auxiliary Encoder:} Scaled by $0.5\times$ to allow moderate adaptation.
    \item \textbf{Fusion Decoder:} Scaled by $1.0\times$ (base LR) to fully learn the segmentation task from scratch.
\end{itemize}
A \textbf{Cosine Annealing} scheduler is used to decay the learning rate smoothly over \textbf{30 epochs}.

\paragraph{Loss Function and Precision.} The model is trained using standard \textbf{Binary Cross Entropy (BCE)} loss. We utilize \textbf{16-bit mixed precision} training to optimize memory usage and throughput, allowing for a batch size of 16 on the $256 \times 256$ inputs.

\paragraph{Data Augmentation.} To improve generalization and robustness against varying satellite imaging conditions, we apply a comprehensive set of augmentations during training:
\begin{itemize}
    \item \textbf{Geometric:} Random discrete rotations ($0^{\circ}, 90^{\circ}, 180^{\circ}, 270^{\circ}$) and random horizontal/vertical flips.
    \item \textbf{Photometric:} Color jittering (adjusting brightness, contrast, saturation, and hue), Gaussian blur, and random image darkening to simulate different lighting conditions and sensor qualities.
\end{itemize}

\section{Extended Experimental Analysis}

\subsection{Runtime Analysis and Resolution Scalability}

Distinct from feed-forward networks that perform single-pass inference, DOGE employs an iterative optimization process to ensure topological precision. While this test-time optimization naturally entails higher latency, it does not demand specialized high-performance computing clusters. On a standard consumer-grade NVIDIA RTX 4090 GPU, optimizing a single $512 \times 512$ tile takes approximately 99 seconds.

Crucially, since the optimization of each tile is mathematically independent, our framework is highly amenable to parallelization. We leverage this by executing 6 concurrent optimization processes on a single GPU during inference. The results reported in \cref{tab:runtime_ablation} reflect the total wall-clock time required to process the entire test set under this parallel setting.

To further evaluate the trade-off between efficiency and precision, we experimented with a reduced resolution of $256 \times 256$. As shown in the table, this setting reduces the total inference time by approximately 43\%, decreasing the aggregate processing time from 302 minutes to 173 minutes. The quantitative results indicate that the performance degradation is negligible, suggesting that the $256 \times 256$ configuration is a highly efficient alternative for throughput-sensitive applications.

\begin{table}[h]
    \centering
    \small
    \caption{Runtime and performance scalability on SpaceNet. The ``Total Time'' represents the wall-clock time to process the full test set using 6 parallel processes on a single RTX 4090.}
    \label{tab:runtime_ablation}
    \setlength{\tabcolsep}{5pt}
    \begin{tabular}{c c c c}
        \toprule
        \textbf{Setting} & \textbf{Resolution} & \textbf{Total Time} & \textbf{F1 / APLS} \\
        \midrule
        High-Fidelity & $512 \times 512$ & 302 min & \textbf{84.6} / \textbf{73.5} \\
        Efficiency & $256 \times 256$ & \textbf{173 min} & 83.7 / 72.6 \\
        \bottomrule
    \end{tabular}
\end{table}

\subsection{Compactness Analysis on SpaceNet}
\label{subsec:spacenet_compactness}

We extend the compactness analysis to the SpaceNet dataset, evaluating the trade-off between topological fidelity (TOPO F1) and graph sparsity (edges/km).

\begin{figure}[h]
    \centering
    \includegraphics[width=0.95\linewidth]{assets/edge density1120_spacenet.pdf}
    \caption{Performance versus compactness on the SpaceNet dataset. The plot illustrates TOPO F1 scores against edge density (edges/km). \textit{DOGE} consistently achieves high topological accuracy while maintaining a significantly lower edge density compared to other methods, underscoring the efficiency of our B\'{e}zier graph representation.}
    \label{fig:spacenet_edge_density}
\end{figure}

As shown in \cref{fig:spacenet_edge_density}, \textit{DOGE} demonstrates a superior balance between performance and compactness. While maintaining state-of-the-art TOPO F1 scores, our method uses substantially fewer edges per kilometer than polyline-based baselines. This efficiency stems from the B\'{e}zier curve's ability to model complex road geometries with minimal control points, avoiding the dense node sampling required by traditional approaches.

\subsection{Cross-Dataset Generalization (Dataset-Agnostic SAM2 + DOGE)}

To evaluate the generalization capability of our framework, we conduct a cross-dataset transfer experiment. Specifically, we train our SAM2-based segmentation model solely on the \textbf{City-Scale} dataset~\cite{heSat2GraphRoadGraph2020} and test it directly on the recently introduced \textbf{Global-Scale Road Dataset} (SAMRoad++)~\cite{Yin_TowardsSatelliteImage_2025}, without any fine-tuning or adaptation on the target domain.

\begin{figure*}[t]
    \centering
    \begin{tikzpicture}
        \node[anchor=south west, inner sep=0] (image) at (0,0) {\includegraphics[width=\linewidth]{assets/fig_globescale.pdf}};
        \begin{scope}[x={(image.south east)},y={(image.north west)}]
            % Assuming 4 columns: GT | Ours | GT | Ours
            % Adjust x-coordinates (0.125, 0.375, 0.625, 0.875) to center text under each column
            \node[font=\small] at (0.125, -0.02) {Ground Truth};
            \node[font=\small] at (0.375, -0.02) {Ours (Cross-Dataset)};
            \node[font=\small] at (0.625, -0.02) {Ground Truth};
            \node[font=\small] at (0.875, -0.02) {Ours (Cross-Dataset)};
        \end{scope}
    \end{tikzpicture}
    \vspace{-2mm}
    \caption{Qualitative results of cross-dataset generalization. The model is trained on City-Scale and tested on the Global-Scale Road Dataset~\cite{Yin_TowardsSatelliteImage_2025} without any fine-tuning. Despite the domain shift and diverse scenes (urban, rural, highways), DOGE successfully reconstructs complete and topologically correct road networks using the same hyperparameters as in the main experiments.}
    \label{fig:globescale_qualitative}
\end{figure*}

\paragraph{Qualitative Analysis.}
The qualitative results are presented in \cref{fig:globescale_qualitative}. Despite the significant domain shift and the diversity of scenes in the Global-Scale dataset---ranging from dense urban grids to rural highways---our method demonstrates remarkable robustness. The SAM2 backbone effectively segments road regions in unseen environments, leveraging its strong dataset-agnostic generalization capabilities. Subsequently, DOGE optimizes the B\'{e}zier graph to fit these predictions, producing smooth and connected road networks.

\paragraph{Robustness of DOGE.}
Crucially, throughout this experiment, we maintain the \textbf{exact same set of hyperparameters} for DOGE (both \textit{DiffAlign} and \textit{TopoAdapt}) as used in our main experiments on SpaceNet and City-Scale. We do not adjust thresholds like the merge distance ($\epsilon_{\text{merge}}=4.0$m) or the collinear angle ($\theta_{\text{collinear}}=170^{\circ}$). The successful reconstruction on this new dataset underscores that our geometric and topological priors are not overfitted to specific datasets but capture intrinsic properties of road networks.

\paragraph{Future Potential.}
This experiment highlights the modular advantage of our framework. As foundation models for segmentation continue to advance, DOGE can be seamlessly paired with them to achieve high-quality, training-free vector topology reconstruction across an ever-widening range of domains and applications.

\begin{figure}[!ht]
    \centering
    \begin{tikzpicture}
        \node[anchor=south west, inner sep=0] (image) at (0,0) {\includegraphics[width=0.95\linewidth]{assets/fig_svanilla_sam.pdf}};
        \begin{scope}[x={(image.south east)},y={(image.north west)}]
            % Assuming 2 columns: GT | Ours
            \node[font=\small] at (0.25, -0.02) {Ground Truth};
            \node[font=\small] at (0.75, -0.02) {Ours (Training-Free)};
        \end{scope}
    \end{tikzpicture}
    \vspace{-2mm}
    \caption{Qualitative results using an off-the-shelf, training-free SAM2 backbone on SpaceNet. We use the raw SAM2 model for zero-shot segmentation followed by DOGE optimization. While the lack of fine-tuning leads to some fragmentation, DOGE still successfully recovers the global topology without any dataset-specific supervision.}
    \label{fig:vanilla_sam_qualitative}
\end{figure}

\begin{figure}[!ht]
    \centering
    \begin{tikzpicture}
        \node[anchor=south west, inner sep=0] (image) at (0,0) {\includegraphics[width=0.95\linewidth]{assets/fig_lanegnn.pdf}};
        \begin{scope}[x={(image.south east)},y={(image.north west)}]
            % Assuming 2 columns: GT | Ours
            \node[font=\small] at (0.25, -0.02) {Ground Truth};
            \node[font=\small] at (0.75, -0.02) {Ours (LaneGNN)};
        \end{scope}
    \end{tikzpicture}
    \vspace{-2mm}
    \caption{Qualitative results on the LaneGNN dataset~\cite{buchnerLearningAggregatingLane2023a}. We apply DOGE to reconstruct lane-level graphs from fine-tuned SAM2 segmentation. The results demonstrate that our B\'{e}zier-based optimization effectively captures the smooth geometry and topology of urban lanes, confirming the framework's adaptability to HD map scenarios.}
    \label{fig:lanegnn_qualitative}
\end{figure}

\begin{figure*}[!t]
    \centering
    \begin{tikzpicture}
        \node[anchor=south west,inner sep=0] (image) at (0,0) {\includegraphics[width=\linewidth]{assets/fig_cityscale_more.pdf}};
        \begin{scope}[x={(image.south east)},y={(image.north west)}]
            \node at (0.12, -0.015) {Ground Truth};
            \node at (0.38, -0.015) {Ours};
            \node at (0.63, -0.015) {Ground Truth};
            \node at (0.88, -0.015) {Ours};
        \end{scope}
    \end{tikzpicture}
    \caption{Additional qualitative comparisons on the City-Scale dataset. Our method faithfully reconstructs complex road topologies and geometries.}
    \label{fig:cityscale_more}
\end{figure*}

\subsection{Training-Free Segmentation Backbone (Off-the-shelf SAM2 + DOGE)}

To evaluate the potential of our framework for fully automated, annotation-free deployment, we conduct an experiment using a \textbf{training-free} segmentation backbone. Specifically, we employ the off-the-shelf \textbf{SAM2}~\cite{raviSAM2Segment2024} model directly on the SpaceNet dataset without any fine-tuning or adaptation to satellite imagery. DOGE is then applied to optimize the B\'{e}zier graph solely based on these zero-shot segmentation predictions.

\paragraph{Results and Discussion.}
Qualitative results are presented in \cref{fig:vanilla_sam_qualitative}. We visualize the ground truth (left) and the reconstruction result from our training-free pipeline (right). 
As expected, the reconstruction quality is lower compared to our fully supervised baseline. The off-the-shelf SAM2 model, untrained on remote sensing data, produces masks with rougher boundaries and occasional fragmentation due to occlusions (e.g., trees or shadows). These segmentation artifacts propagate to the optimization stage, resulting in some noisy, short road segments or disconnected paths.

\paragraph{Conclusion.}
Despite these imperfections, the system successfully recovers the core topological structure of the road network. This experiment serves as a powerful proof-of-concept: \textbf{DOGE does not inherently depend on dataset-specific vector supervision}. Its performance is bounded primarily by the quality of the input segmentation. As foundation models for segmentation continue to evolve and improve in zero-shot precision, DOGE is positioned to unlock high-quality, training-free vector map construction across diverse domains.

\subsection{Generalization to HD Map Scenes (Lane-level)}

To demonstrate the versatility of our framework beyond aerial remote sensing, we extend DOGE to the challenging task of high-definition (HD) map construction for autonomous driving. Specifically, we tackle lane graph reconstruction on the \textbf{LaneGNN} dataset (UrbanLaneGraph)~\cite{buchnerLearningAggregatingLane2023a}.

\paragraph{Experimental Setup.}
We fine-tune SAM2 on the LaneGNN training set to generate lane-level segmentation masks. These masks then serve as the sole supervision for DOGE, which optimizes a B\'{e}zier graph to reconstruct the lane network. This setup tests DOGE's ability to model the complex, curvilinear geometry of urban lanes, which differs significantly from satellite road networks in scale and perspective.

\paragraph{Results and Conclusion.}
Qualitative results are shown in \cref{fig:lanegnn_qualitative}, comparing the ground truth lane graph (left) with our reconstructed B\'{e}zier lane graph (right). DOGE successfully produces smooth, high-fidelity lane curves that accurately follow the driving corridors. 
This experiment confirms that DOGE is not limited to satellite imagery but is a generic solver for vector topology reconstruction. Whether for macroscopic road networks or microscopic HD lanes, our curve-based optimization framework demonstrates a broad applicability to geometric feature extraction tasks across different domains.

\subsection{Additional Qualitative Comparisons}

We provide more qualitative results on the City-Scale dataset in \cref{fig:cityscale_more}.
